# Supplementary material for: HO-Cap: A Capture System and Dataset for 3D Reconstruction and Pose Tracking of Hand-Object Interaction
Source: arXiv:2406.06843 source file (2025-03-11)

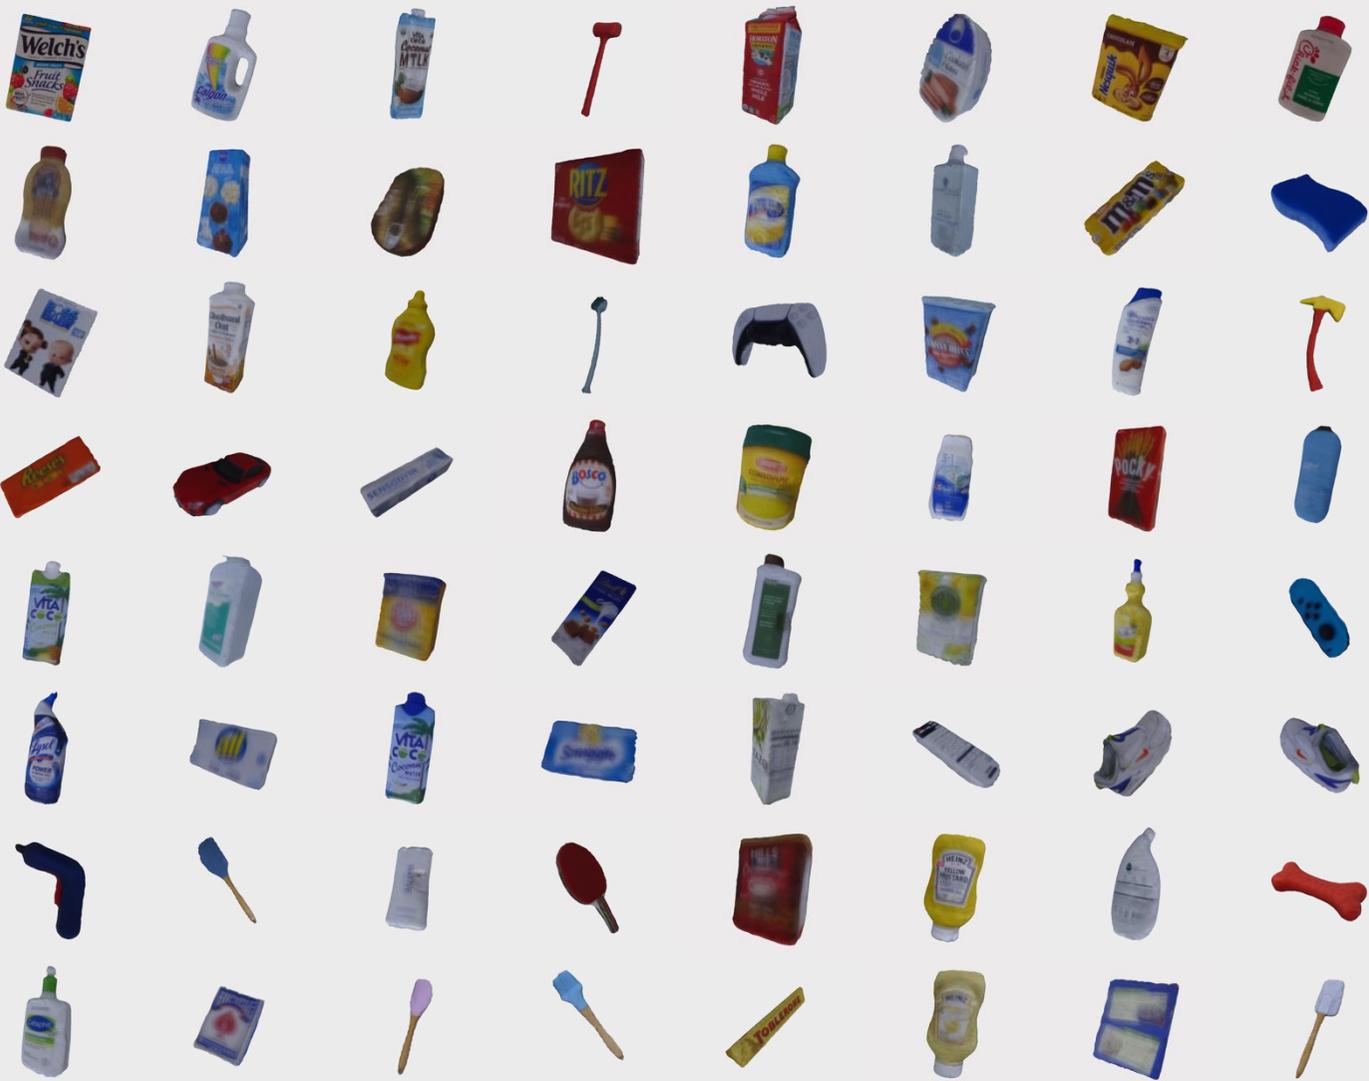

Supplement: Supplementary file 1 [file supp_fig_all_models.pdf]
